# Supplementary material for: An Efficient scaled opposite-spin MP2 method for periodic systems
Source: arXiv:2503.20482 source file (2025-03-26)
Supplement: Supplementary file 1 [file SI_Efficient_spin_opposite_scale_MP2_methods_for_periodic_systems___submission.pdf]

# Supporting Information for: An Efficient scaled opposite-spin MP2 method for periodic systems

Idan Haritan,† Xiao Wang,*,‡ and Tamar Goldzak*,†

†*The Alexander Kofkin Faculty of Engineering, Bar-Ilan University, Ramat Gan 52900, Israel*

‡*Department of Chemistry and Biochemistry, University of California Santa Cruz, Santa Cruz, CA 95064, United States*

E-mail: xwang431@ucsc.edu; tamar.goldzak@biu.ac.il

To evaluate the performance of the three quadrature algorithms discussed in the main text, i.e., (1) the original algorithm proposed by Haser and Almlöf,[1] (2) the logarithmic transformed algorithm proposed by Ayala, Kudin, and Scuseria,[2] and (3) the minimax algorithm proposed by Takatsuka, Ten-no, and Hackbusch,[3] we compared correlation energies computed from conventional MP2 with resolution of the identity (RI-MP2) and Laplace transformed RI-MP2 (RILT-MP2). These algorithms are referred to as Almlöf, Scuseria, and Hackbusch, respectively, for brevity. Since this analysis focused on the accuracy of different quadrature algorithms in LT, the scaled opposite-spin (SOS) approximation was not used. This analysis was conducted for five monomers from the S22 dataset:[4] ammonia ($NH_3$), water ($H_2O$), formic acid ($CH_2O_2$), formamide ($CH_3NO$), and uracil ($C_4H_4N_2O_2$). For each molecule, the number of quadrature points was varied in RILT-MP2, and the corresponding correlation energies ($E^{\text{corr}}_{\text{RILT-MP2}}$) were recorded, in comparison to the reference energy $E^{\text{corr}}_{\text{RI-MP2}}$. Dunning's cc-pVTZ basis set[5] was used for all molecules. Tab. S1 summarize these results, illustrating the trade-off between the number of quadrature points and the accuracy of the computed energies. The Hackbusch method consistently demonstrated superior accuracy with fewer grid points, confirming its efficiency and suitability for the development

of Laplace transformed MP2, including the SOS-RILT-MP2 method proposed in this work.

Building on the insights from the molecular systems, we extended our analysis to a periodic system, applying the quadrature methods to a diamond crystal using a 2×2×2 k-point grid with the GTH pseudopotential and the corresponding SZV basis set. The results for the Almlöf, Scuseria, and Hackbusch methods are presented in Table S2.

Table S1: Comparison of quadrature methods for RILT-MP2 on selected molecules from the S22 dataset. The table lists the molecule, quadrature method, number of quadrature points applied, the RI-MP2 correlation energy ($E^{\text{corr}}_{\text{RI-MP2}}$), the RILT-MP2 correlation energy ($E^{\text{corr}}_{\text{RILT-MP2}}$), and the energy deviation ($\Delta E$) between the two methods. Energies are reported in Hartree.

| **Molecule** | **Method** | **Quadrature points** | $\mathbf{E^{corr}_{RI-MP2}}$ | $\mathbf{E^{corr}_{RILT-MP2}}$ | **ΔE** |
|---|---|---|---|---|---|
| $NH_3$ | Scuseria | 3 | -0.250036191559 | -0.238163643742 | 1.19e-02 |
| $NH_3$ | Scuseria | 4 | -0.250036191559 | -0.243878757088 | 6.16e-03 |
| $NH_3$ | Scuseria | 5 | -0.250036191559 | -0.247177195720 | 2.86e-03 |
| $NH_3$ | Scuseria | 6 | -0.250036191559 | -0.248902846720 | 1.13e-03 |
| $NH_3$ | Scuseria | 7 | -0.250036191559 | -0.249653219833 | 3.83e-04 |
| $NH_3$ | Scuseria | 8 | -0.250036191559 | -0.249926326855 | 1.10e-04 |
| $NH_3$ | Scuseria | 9 | -0.250036191559 | -0.250009870296 | 2.63e-05 |
| $NH_3$ | Scuseria | 10 | -0.250036191559 | -0.250031313322 | 4.88e-06 |
| $NH_3$ | Almlöf | 3 | -0.250036191559 | -0.249674686817 | 3.62e-04 |
| $NH_3$ | Almlöf | 4 | -0.250036191559 | -0.249917682621 | 1.19e-04 |
| $NH_3$ | Almlöf | 5 | -0.250036191559 | -0.250035956434 | 2.35e-07 |
| $NH_3$ | Almlöf | 6 | -0.250036191559 | -0.250034400789 | 1.79e-06 |
| $NH_3$ | Almlöf | 7 | -0.250036191559 | -0.250035696120 | 4.95e-07 |
| $NH_3$ | Almlöf | 8 | -0.250036191559 | -0.250036090950 | 1.01e-07 |
| $NH_3$ | Almlöf | 9 | -0.250036191559 | -0.250036054622 | 1.37e-07 |
| $NH_3$ | Almlöf | 10 | -0.250036191559 | -0.250034266349 | 1.93e-06 |
| $NH_3$ | Hackbusch | 5 | -0.250036170312 | -0.250049109012 | -1.29e-05 |
| $NH_3$ | Hackbusch | 6 | -0.250036170312 | -0.250039719238 | -3.55e-06 |
| $NH_3$ | Hackbusch | 7 | -0.250036170312 | -0.250036071956 | 9.84e-08 |
| $H_2O$ | Scuseria | 3 | -0.275311448354 | -0.262977725176 | 1.23e-02 |
| $H_2O$ | Scuseria | 4 | -0.275311448354 | -0.269486584678 | 5.82e-03 |
| $H_2O$ | Scuseria | 5 | -0.275311448354 | -0.272709685094 | 2.60e-03 |
| $H_2O$ | Scuseria | 6 | -0.275311448354 | -0.274307421779 | 1.00e-03 |
| $H_2O$ | Scuseria | 7 | -0.275311448354 | -0.274980488892 | 3.31e-04 |
| $H_2O$ | Scuseria | 8 | -0.275311448354 | -0.275219389137 | 9.21e-05 |
| $H_2O$ | Scuseria | 9 | -0.275311448354 | -0.275290427733 | 2.10e-05 |
| $H_2O$ | Scuseria | 10 | -0.275311448354 | -0.275307964875 | 3.48e-06 |
| $H_2O$ | Almlöf | 3 | -0.275311448354 | -0.274960384632 | 3.51e-04 |
| $H_2O$ | Almlöf | 4 | -0.275311448354 | -0.275225218635 | 8.62e-05 |

| | | | | | |
|---|---|---|---|---|---|
| $H_2O$ | Almlöf | 5 | -0.275311448354 | -0.275301777907 | 9.67e-06 |
| $H_2O$ | Almlöf | 6 | -0.275311448354 | -0.275312145945 | -6.98e-07 |
| $H_2O$ | Almlöf | 7 | -0.275311448354 | -0.275312840617 | -1.39e-06 |
| $H_2O$ | Almlöf | 8 | -0.275311448354 | -0.275312799790 | -1.35e-06 |
| $H_2O$ | Almlöf | 9 | -0.275311448354 | -0.275312061315 | -6.13e-07 |
| $H_2O$ | Almlöf | 10 | -0.275311448354 | -0.275311902863 | -4.55e-07 |
| $H_2O$ | Hackbusch | 5 | -0.275311448772 | -0.275315180416 | -3.73e-06 |
| $H_2O$ | Hackbusch | 6 | -0.275311448772 | -0.275317076566 | -5.63e-06 |
| $H_2O$ | Hackbusch | 7 | -0.275311448772 | -0.275311345420 | 1.03e-07 |
| $CH_2O_2$ | Scuseria | 3 | -0.672989783180 | -0.637993828298 | 3.50e-02 |
| $CH_2O_2$ | Scuseria | 4 | -0.672989783180 | -0.656406623771 | 1.66e-02 |
| $CH_2O_2$ | Scuseria | 5 | -0.672989783180 | -0.665604556807 | 7.39e-03 |
| $CH_2O_2$ | Scuseria | 6 | -0.672989783180 | -0.670116186802 | 2.87e-03 |
| $CH_2O_2$ | Scuseria | 7 | -0.672989783180 | -0.672019365142 | 9.70e-04 |
| $CH_2O_2$ | Scuseria | 8 | -0.672989783180 | -0.672709618333 | 2.80e-04 |
| $CH_2O_2$ | Scuseria | 9 | -0.672989783180 | -0.672924234733 | 6.55e-05 |
| $CH_2O_2$ | Scuseria | 10 | -0.672989783180 | -0.672980562520 | 9.22e-06 |
| $CH_2O_2$ | Almlöf | 3 | -0.672989783180 | -0.672220356103 | 7.69e-04 |
| $CH_2O_2$ | Almlöf | 4 | -0.672989783180 | -0.672911879084 | 7.79e-05 |
| $CH_2O_2$ | Almlöf | 5 | -0.672989783180 | -0.672973391058 | 1.64e-05 |
| $CH_2O_2$ | Almlöf | 6 | -0.672989783180 | -0.672992197168 | -2.41e-06 |
| $CH_2O_2$ | Almlöf | 7 | -0.672989783180 | -0.672989587950 | 1.95e-07 |
| $CH_2O_2$ | Almlöf | 8 | -0.672989783180 | -0.672990243524 | -4.60e-07 |
| $CH_2O_2$ | Almlöf | 9 | -0.672989783180 | -0.672989922543 | -1.39e-07 |
| $CH_2O_2$ | Almlöf | 10 | -0.672989783180 | -0.672989607525 | 1.76e-07 |
| $CH_2O_2$ | Hackbusch | 5 | -0.672989688666 | -0.672981819288 | 7.87e-06 |
| $CH_2O_2$ | Hackbusch | 6 | -0.672989688666 | -0.672997100735 | 7.41e-06 |
| $CH_2O_2$ | Hackbusch | 7 | -0.672989688666 | -0.672990313420 | 6.25e-07 |
| $CH_3NO$ | Scuseria | 3 | -0.648628590603 | -0.611378878160 | 3.72e-02 |
| $CH_3NO$ | Scuseria | 4 | -0.648628590603 | -0.629965254932 | 1.87e-02 |
| $CH_3NO$ | Scuseria | 5 | -0.648628590603 | -0.639880973636 | 8.75e-03 |
| $CH_3NO$ | Scuseria | 6 | -0.648628590603 | -0.645040546196 | 3.59e-03 |
| $CH_3NO$ | Scuseria | 7 | -0.648628590603 | -0.647343383789 | 1.29e-03 |
| $CH_3NO$ | Scuseria | 8 | -0.648628590603 | -0.648227669982 | 4.01e-04 |
| $CH_3NO$ | Scuseria | 9 | -0.648628590603 | -0.648521711279 | 1.07e-04 |
| $CH_3NO$ | Scuseria | 10 | -0.648628590603 | -0.648606202591 | 2.24e-05 |
| $CH_3NO$ | Almlöf | 3 | -0.648628590603 | -0.648139223792 | 4.89e-04 |
| $CH_3NO$ | Almlöf | 4 | -0.648628590603 | -0.648587168879 | 4.14e-05 |
| $CH_3NO$ | Almlöf | 5 | -0.648628590603 | -0.648645400911 | -1.68e-05 |
| $CH_3NO$ | Almlöf | 6 | -0.648628590603 | -0.648630985569 | -2.39e-06 |
| $CH_3NO$ | Almlöf | 7 | -0.648628590603 | -0.648628536796 | 5.38e-08 |
| $CH_3NO$ | Almlöf | 8 | -0.648628590603 | -0.648628399615 | 1.91e-07 |

| | | | | | |
|---|---|---|---|---|---|
| $CH_3NO$ | Almlöf | 9 | -0.648628590603 | -0.648629671144 | -1.08e-06 |
| $CH_3NO$ | Almlöf | 10 | -0.648628590603 | -0.648628390924 | 2.00e-07 |
| $CH_3NO$ | Hackbusch | 5 | -0.648628431188 | -0.648642637295 | 1.42e-05 |
| $CH_3NO$ | Hackbusch | 6 | -0.648628431188 | -0.648633119088 | 4.69e-06 |
| $CH_3NO$ | Hackbusch | 7 | -0.648628431188 | -0.648627948986 | 4.82e-07 |
| $C_4H_4N_2O_2$ | Scuseria | 3 | -1.592305851145 | -1.473584616858 | 1.19e-01 |
| $C_4H_4N_2O_2$ | Scuseria | 4 | -1.592305851145 | -1.529651801840 | 6.27e-02 |
| $C_4H_4N_2O_2$ | Scuseria | 5 | -1.592305851145 | -1.560003747487 | 3.23e-02 |
| $C_4H_4N_2O_2$ | Scuseria | 6 | -1.592305851145 | -1.577358690935 | 1.49e-02 |
| $C_4H_4N_2O_2$ | Scuseria | 7 | -1.592305851145 | -1.586132117831 | 6.17e-03 |
| $C_4H_4N_2O_2$ | Scuseria | 8 | -1.592305851145 | -1.590017571763 | 2.29e-03 |
| $C_4H_4N_2O_2$ | Scuseria | 9 | -1.592305851145 | -1.591543065966 | 7.63e-04 |
| $C_4H_4N_2O_2$ | Scuseria | 10 | -1.592305851145 | -1.592078204170 | 2.28e-04 |
| $C_4H_4N_2O_2$ | Almlöf | 3 | -1.592305851145 | -1.590669501617 | 1.64e-03 |
| $C_4H_4N_2O_2$ | Almlöf | 4 | -1.592305851145 | -1.592706147219 | -4.00e-04 |
| $C_4H_4N_2O_2$ | Almlöf | 5 | -1.592305851145 | -1.592335903143 | -3.01e-05 |
| $C_4H_4N_2O_2$ | Almlöf | 6 | -1.592305851145 | -1.592301349565 | 4.50e-06 |
| $C_4H_4N_2O_2$ | Almlöf | 7 | -1.592305851145 | -1.592304304251 | 1.55e-06 |
| $C_4H_4N_2O_2$ | Almlöf | 8 | -1.592305851145 | -1.592305027040 | 8.24e-07 |
| $C_4H_4N_2O_2$ | Almlöf | 9 | -1.592305851145 | -1.592305727969 | 1.23e-07 |
| $C_4H_4N_2O_2$ | Almlöf | 10 | -1.592305851145 | -1.592303741738 | 2.11e-06 |
| $C_4H_4N_2O_2$ | Hackbusch | 5 | -1.592305654143 | -1.592348202444 | 4.25e-05 |
| $C_4H_4N_2O_2$ | Hackbusch | 6 | -1.592305654143 | -1.592308972755 | 3.32e-06 |
| $C_4H_4N_2O_2$ | Hackbusch | 7 | -1.592305654143 | -1.592305076142 | 5.78e-07 |

Table S2: Comparison of quadrature methods for the RILT-MP2 in a periodic diamond system using a $2 \times 2 \times 2$ k-point grid and the GTH/SZV pseudopotential/basis set. The table lists the method, number of quadrature points applied, the RI-MP2 correlation energy ($E^{\mathrm{corr}}_{\mathrm{RI-MP2}}$), the RILT-MP2 correlation energy ($E^{\mathrm{corr}}_{\mathrm{RILT-MP2}}$), and the energy deviation ($\Delta E$) between the two methods. Energies are reported in Hartree.

| Method | Quadrature points | $\mathbf{E^{corr}_{RI-MP2}}$ | $\mathbf{E^{corr}_{RILT-MP2}}$ | ΔE |
|---|---|---|---|---|
| Scuseria | 3 | -0.094877933246 | -0.095178219523 | -3.00e-04 |
| Scuseria | 4 | -0.094877933246 | -0.095027599401 | -1.50e-04 |
| Scuseria | 5 | -0.094877933246 | -0.094964074436 | -8.61e-05 |
| Scuseria | 6 | -0.094877933246 | -0.094932353265 | -5.44e-05 |
| Scuseria | 7 | -0.094877933246 | -0.094914635175 | -3.67e-05 |
| Almlöf | 3 | -0.094877933246 | -0.094872480007 | 5.45e-06 |
| Almlöf | 4 | -0.094877933246 | -0.094871568968 | 6.36e-06 |
| Almlöf | 5 | -0.094877933246 | -0.094874061749 | 3.87e-06 |
| Almlöf | 6 | -0.094877933246 | -0.094876200809 | 1.73e-06 |
| Almlöf | 7 | -0.094877933246 | -0.094876916858 | 1.02e-06 |
| Hackbusch | 5 | -0.094877930842 | -0.094877862844 | 6.80e-08 |
| Hackbusch | 6 | -0.094877930842 | -0.094877922986 | 7.86e-09 |

# References


(1) Häser, M.; Almlöf, J. Laplace transform techniques in Mo/ller–Plesset perturbation theory. *The Journal of chemical physics* **1992**, *96*, 489–494.

(2) Ayala, P. Y.; Kudin, K. N.; Scuseria, G. E. Atomic orbital Laplace-transformed second-order Møller–Plesset theory for periodic systems. *The Journal of Chemical Physics* **2001**, *115*, 9698–9707.

(3) Takatsuka, A.; Ten-No, S.; Hackbusch, W. Minimax approximation for the decomposition of energy denominators in Laplace-transformed Møller–Plesset perturbation theories. *The Journal of chemical physics* **2008**, *129*.

(4) Jurečka, P.; Šponer, J.; Černỳ, J.; Hobza, P. Benchmark database of accurate (MP2 and CCSD (T) complete basis set limit) interaction energies of small model complexes, DNA base pairs, and amino acid pairs. *Physical Chemistry Chemical Physics* **2006**, *8*, 1985–1993.

(5) Dunning Jr, T. H. Gaussian basis sets for use in correlated molecular calculations. I. The atoms boron through neon and hydrogen. *The Journal of chemical physics* **1989**, *90*, 1007–1023.
